# Supplementary material for: Multiple Abstraction Level Retrieve Augment Generation
Source: arXiv:2501.16952 source file (2025-01-28)
Supplement: Supplementary file 1 [file Supplementary_Materials.pdf]

# Supplementary Materials

## A. PROMPTS FOR SECTION AND DOCUMENT SUMMARY GENERATION

This section provides details on generating section summary chunks and document summary chunks. The same prompt is used for all summary tasks, as they involve summarizing a group of contexts in a similar manner.

### SUMMARIZATION PROMPT:

**System:** You are an advanced language model designed to provide expert, high-quality responses. Your task is to understand the user’s input and generate an appropriate response.

**User:** You are an expert academic researcher. Generate an abstractive summary of the given research content. Limit the number of sentences in the summary to a maximum of three.

-----  
Here is the content:

{context\_str}

-----  
**Response:**

{context\_str} represents the content to be summarized. In section-level summarization, it consists of paragraphs from the corresponding section, whereas in document-level summarization, it comprises section summaries of the entire document. Thus, the contexts to be summarized are structured as a list of texts.

When executing the summarization task, we encounter two primary challenges. First, the text to be summarized can be excessively long. Second, the generated summary may exceed the length constraints.

To address the first challenge, we apply the summarization prompt to each text individually, generating a condensed version for each unit—paragraph summaries for section-level summarization and section summaries for document-level summarization. To further handle the length limitation in LLM, we divide the summaries that we just generate into groups that fit within the token limit of the LLM and summarize each group separately. This process is repeated iteratively, grouping and summarizing the results, until only a single final paragraph remains.

For the section problem, we employ an iterative refinement process to reduce the number of sentences while preserving key information. The refinement process is executed a predefined number of times to approach conciseness requirement. In our work, it is 10. This process terminates when the summary meets the required length or when the refinement limit is reached, indicating that the content contains rich information that necessitates a longer summary.

**SUMMARIZATION PROMPT:**

System: You are an advanced language model designed to provide expert, high-quality responses. Your task is to understand the user's input and generate an appropriate response.

User: You are an expert researcher. Generate an abstractive summary of one or two most important points from the given text. Start with a numbered list format, like '1.' and '2.'.

-----  
Here is the content:

{context\_str}

-----  
Response:

**B. PROMPTS FOR QUESTION ANSWER AND REASON(QAR) PAIRS GENERATION**

This section discusses the prompt used for Question Answer evaluation dataset generation. In this process, we designed pydantic model and QAR templates based on LangChain package<sup>1</sup>.

Pydantic model:

Defining a Pydantic model for QAR GENERATION PROMPT.

```
class QAR(BaseModel):
    Reason: str = Field(description="The reason for the answer")
    Question: str = Field(description="The question being asked")
    Answer: str = Field(description="The answer to the question")

class MultipleQARs(BaseModel):
    qars: list[QAR]
```

This code serves as a template that will be converted into JSON format for the QAR Generation Prompt.

---

<sup>1</sup>PromptTemplate: [https://api.python.langchain.com/en/latest/prompts/langchain\\_core.prompts.prompt.PromptTemplate.html](https://api.python.langchain.com/en/latest/prompts/langchain_core.prompts.prompt.PromptTemplate.html)

**QAR GENERATION PROMPT:**

Based on the provided context, simulate how researchers might generate {qar\_num} academic questions and find corresponding references to answer them. Each question should be something that can be directly answered by the context provided. Answer each question using only the information from the context, limiting answers to three sentences. Finally, explain why each question is important and how the context serves as the reference to provide the answers.

Context: {context\_str}

-----  
The output should be formatted as a JSON instance that conforms to the JSON schema below.

As an example, for the schema {"properties": {"foo": {"title": "Foo", "description": "a list of strings", "type": "array", "items": {"type": "string"}}}, "required": ["foo"]}

the object {"foo": ["bar", "baz"]} is a well-formatted instance of the schema. The object {"properties": {"foo": ["bar", "baz"]}} is not well-formatted.

Here is the output schema:

```
"""
{"properties": {"qars": {"title": "Qars", "type": "array", "items": {"$ref": "#definitionsQAR"}},
"required": ["qars"], "definitions": {"QAR": {"title": "QAR", "type": "object", "properties":
{"Reason": {"title": "Reason", "description": "The reason for the answer", "type": "string"},
"Question": {"title": "Question", "description": "The question being asked", "type":
"string"}, "Answer": {"title": "Answer", "description": "The answer to the question",
"type": "string"}}, "required": ["Reason", "Question", "Answer"]}}}
"""
```

Output a valid JSON object but do not repeat the schema.

{qar\_num} denotes the number of QAR pairs to be generated, while {context\_str} represents the context from the chunks used for generating the QAR pairs.
